# Supplementary material for: Parse, Search, and Confirmation: Training-Free Aerial Vision-and-Dialog Navigation with Chain-of-Thought Reasoning and Structured Spatial Memory
Source: arXiv:2607.11529 source file (2026-07-13)
Supplement: Supplementary file 1 [file supp.tex]

\clearpage
\setcounter{page}{1}
\maketitlesupplementary

\section{More Dataset Details}
\label{sec:Dataset Details}
To provide a more comprehensive background on the ANDH~\cite{Fan22} and ANDH-Full~\cite{Fan22} datasets used in this experiment, we elaborate on their data composition and collection design.
Both datasets are derived from the AVDN base dataset~\cite{Fan22}, which is constructed using a customized UAV simulator that generates an original georeferenced map by cropping X-View satellite imagery.
Each map corresponds to a fixed real-world area, accurately preserving realistic aerial visual characteristics.
Specifically, the dataset contains $3,064$ full navigation trajectories, each associated with multiple rounds of natural language dialogue.
These trajectories are further segmented into $6,269$ sub-trajectories, each corresponding to a single dialogue cycle.
The average length of a full trajectory is $287$ meters, while sub-trajectories range from $142$ to $148$ meters on average.

\section{More Implementation Details}
\label{sec:Implementation Details}
To map any pixel coordinate $(u,v)$ from the multi-scale visual observation of our SSM module back to its corresponding location on the original georeferenced map, we employ an inverse homography transformation.

First, we compute the inverse homography matrix $H_{\rm{inv}}$ based on the correspondence between the four corners of the visual observation, denoted as $(0,0),(S,0),(0,S),(S,S)$, and their corresponding points $(X_i,Y_i)$ on the original georeferenced map.
Let $H_{\rm{inv}} = [h_{ij}]_{3 \times 3}$.
The relationship between the visual observation coordinates and the homogeneous georeferenced map coordinates is given by:
\begin{equation}
    \begin{bmatrix}
    X \\ Y \\ 1
    \end{bmatrix}
    \propto
    H_{\rm{inv}}
    \begin{bmatrix}
    u \\ v \\ 1
    \end{bmatrix}.
\end{equation}

Specifically, the Cartesian pixel coordinates $(X,Y)$ on the georeferenced map are obtained via:
\begin{equation}
X =
\frac{
h_{00}u +
h_{01}v +
h_{02}
}{
h_{20}u +
h_{21}v +
h_{22}
},
\end{equation}
\begin{equation}
Y =
\frac{
h_{10}u +
h_{11}v +
h_{12}
}{
h_{20}u +
h_{21}v +
h_{22}
}.
\end{equation}

Finally, we convert $(X,Y)$ to geographic coordinates $(\text{lng},\text{lat})$ using linear interpolation, where lng and lat denotes longitude and latitude, respectively.
The georeferenced map follows a standard image coordinate system with the origin at the top-left corner, whereas the geographic coordinate system is defined from the bottom-left.
Let the georeferenced map have a resolution of $W_{\rm{map}} \times H_{\rm{map}}$, and its geospatial bounds is defined by the lower-left coordinate $(\text{lng}_{\min}, \text{lat}_{\min})$ and the upper-right coordinate $(\text{lng}_{\max}, \text{lat}_{\max})$.
The conversion is defined as:
\begin{equation}
\text{lng}
=
\text{lng}_{\min}
+
\frac{X}{W_{\rm{map}}}
\left(
\text{lng}_{\max} - \text{lng}_{\min}
\right),
\end{equation}
\begin{equation}
\text{lat}
=
\text{lat}_{\max}
-
\frac{Y}{H_{\rm{map}}}
\left(
\text{lat}_{\max} - \text{lat}_{\min}
\right).
\end{equation}

\section{More Ablation Studies}
\label{sec:Ablation Studies}

\newcolumntype{C}[1]{>{\centering\arraybackslash}m{#1}}   % ← p 改成 m，垂直居中
% ---------- Table: image resolution ----------
\begin{table}[!htbp]
\centering
\small
\setlength{\tabcolsep}{1.8pt}

{\setlength{\aboverulesep}{0pt}%
 \setlength{\belowrulesep}{0pt}%
\begin{tabular}{>{\centering\arraybackslash}p{2.8cm} | 
                >{\centering\arraybackslash}m{1.5cm}
                >{\centering\arraybackslash}m{1.5cm}
                >{\centering\arraybackslash}m{1.5cm}}
 \toprule
 \rowcolor{gray!10}
 \textbf{Image resolution} & \textbf{SPL} & \textbf{SR} & \textbf{GP} \\
 \midrule
 512$\times$512   & 15.1 & 19.7 & 38.0 \\
 768$\times$768   & \textbf{17.8} & \textbf{22.6} & \textbf{39.2} \\
 1024$\times$1024 & 16.7 & 20.9 & 36.3 \\
 \bottomrule
 \end{tabular}%
}
\caption{Ablation results of different image resolutions of the main view.}
\label{tab:image_resolution}
\end{table}

As shown in Table~\ref{tab:image_resolution}, we conduct an ablation study on the cropping resolution of the main view by comparing three input sizes: $512 \times 512$, $768 \times 768$, and $1024 \times 1024$. The results indicate that the $768 \times 768$ configuration achieves the best overall performance across all three evaluation metrics. This suggests that lower resolutions tend to lose critical structural details, thereby hindering accurate target localization. In contrast, excessively high resolutions introduce more irrelevant background and noise, and further exacerbate the instability of Qwen's~\cite{Alibaba23} visual encoding and geometric mapping, which ultimately degrades performance. The $768 \times 768$ setting strikes a favorable balance between fine-grained detail preservation and sufficient global context, and is therefore adopted as the default field of view size in all subsequent experiments.

% \newcolumntype{C}[1]{>{\centering\arraybackslash}p{#1}}

% % ---------- Table: image resolution ----------
% \begin{table}[!htbp]
% \centering
% \small
% \setlength{\tabcolsep}{1.8pt}
% \renewcommand{\arraystretch}{1.10}
% {\setlength{\aboverulesep}{0pt}%
%  \setlength{\belowrulesep}{0pt}%
% \begin{tabular}{@{\hspace{1.8pt}} C{2.2cm} | C{1.0cm} C{1.0cm} C{1.0cm} @{\hspace{1.8pt}}}
%  \toprule
%  \rowcolor{gray!10}
%  \textbf{Image resolution} & \textbf{SPL} & \textbf{SR} & \textbf{GP} \\
%  \midrule
%  512$\times$512   & 15.1 & 19.7 & 38.0 \\
%  768$\times$768   & \textbf{17.8} & \textbf{22.6} & \textbf{39.2} \\
%  1024$\times$1024 & 16.7 & 20.9 & 36.3 \\
%  \bottomrule
%  \end{tabular}%
% }
% \caption{Ablation results across different image resolutions.}
% \label{tab:image_resolution}
% \end{table}

\newcolumntype{C}[1]{>{\centering\arraybackslash}m{#1}}   % ← p 改成 m，垂直居中
% ---------- Table: step ----------
\begin{table}[!htbp]
\centering
\small
\setlength{\tabcolsep}{1.8pt}

{\setlength{\aboverulesep}{0pt}%
 \setlength{\belowrulesep}{0pt}%
\begin{tabular}{@{\hspace{1.8pt}} C{2.0cm} | C{1.0cm} C{1.0cm} C{1.0cm} @{\hspace{1.8pt}}}
 \toprule
 \rowcolor{gray!10}
 \textbf{Steps} & \textbf{SPL} & \textbf{SR} & \textbf{GP} \\
 \midrule
 2 & \textbf{17.9} & 20.2 & 38.4 \\
 3 & 17.8 & \textbf{22.6} & \textbf{39.2} \\
 4 & 15.7 & 20.0 & 37.2 \\
 5 & 15.6 & 19.7 & 33.7 \\
 \bottomrule
 \end{tabular}%
}
\caption{Ablation results of different maximum search steps.}
\label{tab:steps}
\end{table}

\begin{table*}[!htbp]
\centering
\small
\setlength{\tabcolsep}{10pt}

\definecolor{tfpink}{RGB}{255,235,240}
\definecolor{tfpink2}{RGB}{255,220,228}

{\setlength{\aboverulesep}{0pt}%
 \setlength{\belowrulesep}{0pt}%

\begin{tabular}{c|ccc ccc ccc}
\toprule

% ---------------- 新增 ANDH 行 ----------------
\rowcolor{gray!10}
\multicolumn{1}{c|}{\cellcolor{gray!10}}
& \multicolumn{9}{c}{\textbf{ANDH}} \\   % ← 下方横线已删除（原来这里是 \midrule）

% ---------------- 原始表头 ----------------
\rowcolor{gray!10}
\textbf{Method}
& \multicolumn{3}{c}{Seen Val.}
& \multicolumn{3}{c}{Unseen Val.}
& \multicolumn{3}{c}{Unseen Test}
\\

\rowcolor{gray!10}
& \textbf{SPL} & \textbf{SR} & \textbf{GP}
& \textbf{SPL} & \textbf{SR} & \textbf{GP}
& \textbf{SPL} & \textbf{SR} & \textbf{GP}
\\

\midrule
GeoGround~\cite{zhou2024geoground}
& 2.8 & 3.0 & -2.5
& 5.6 & 5.6 & -3.8
& 2.8 & 2.8 & -2.3
\\

\midrule
RemoteSAM~\cite{yao2025remotesam}
& 5.3 & 6.2 & 6.6
& 6.1 & 6.3 & 6.8
& 4.8 & 5.0 & 6.1
\\

\midrule
\rowcolor{tfpink2}
\textbf{PSC-AVDN (Ours)}
& \textbf{16.3} & \textbf{18.6} & \textbf{37.4}
& \textbf{17.8} & \textbf{22.6} & \textbf{39.2}
& \textbf{13.5} & \textbf{16.4} & \textbf{28.2}
\\

\bottomrule
\end{tabular}%
}

\caption{Comparison with remote sensing large models on the ANDH dataset for training-free AVDN task.}
\label{tab:andh_results_avdn_only}
\end{table*}

As reported in Table~\ref{tab:steps}, we further conduct an ablation study on the maximum number of search steps by increasing the limit from $2$ to $5$ steps.
The results show that using $3$ steps yields the best overall performance and clearly surpasses both the $2$ step setting and larger step counts.
Although the $2$ step configuration achieves a slightly higher SPL, its SR and GP scores are substantially lower, indicating that insufficient search often forces the agent to stop prematurely before adequate exploration has been completed.
Conversely, when the search limit increases to $4$ or $5$ steps, all three metrics deteriorate, with GP dropping markedly to $33.7$ under the $5$ step setting.
This trend suggests that excessive search depth accumulates geometric drift and decision errors, causing the predicted trajectory to deviate from the true path.
Overall, the $3$ step configuration achieves the best trade-off between sufficient exploration and limiting error accumulation, thereby yielding the most stable navigation performance.

\section{Results of Remote Sensing Large Models}
As shown in Table~\ref{tab:andh_results_avdn_only}, we investigate the performance of MLLM (GeoGround~\cite{zhou2024geoground}) and vision foundation model (RemoteSAM~\cite{yao2025remotesam}) that are specifically trained for remote sensing scenarios when applied to the training-free AVDN task.
The experiments are conducted on the ANDH dataset.
We find that even models specifically trained on remote sensing data still struggle to effectively perform the training-free AVDN task when directly given natural language navigation instructions.
This validates the effectiveness of our proposed three-stage reasoning pipeline and structured spatial memory module.
\section{Results of different MLLMs}
As shown in Table~\ref{tab:4}, applying our PSC-AVDN framework to different MLLMs consistently improves their performances.
This demonstrates the strong generalizability of our proposed CoT reasoning and spatial memory, with the improvement being particularly pronounced on specialized VL models (\textit{e.g.}, Qwen-VL in our paper and Seed-VL).
\begin{table}[!htbp]
\centering
\small
\setlength{\tabcolsep}{4pt}

{\setlength{\aboverulesep}{0pt}%
 \setlength{\belowrulesep}{0pt}%
\begin{tabular}{c|ccc ccc}
\toprule

% ---------- 数据集行 ----------
\rowcolor{gray!10}
\multicolumn{1}{c|}{\cellcolor{gray!10}} & \multicolumn{6}{c}{\textbf{ANDH}} \\

% ---------- 主表头 ----------
\rowcolor{gray!10}
\textbf{Method} & \multicolumn{3}{c}{Seen Val.} & \multicolumn{3}{c}{Unseen Val.} \\

\rowcolor{gray!10}
 & \textbf{SPL} & \textbf{SR} & \textbf{GP} & \textbf{SPL} & \textbf{SR} & \textbf{GP} \\

\midrule

GPT-4o~\cite{Shahriar24} & 2.6 & 2.7 & -9.5 & 3.4 & 3.9 & -11.8 \\

\rowcolor{gray!15}
Ours (GPT-4o) & \textbf{6.0} & \textbf{9.5} & \textbf{27.7} & \textbf{7.6} & \textbf{10.9} & \textbf{35.2} \\

\midrule

Seed-VL~\cite{guo2025seed15vl} & 3.5 & 4.3 & -4.1 & 4.0 & 4.6 & -5.5 \\

\rowcolor{gray!20}
Ours (Seed-VL) & \textbf{10.2} & \textbf{13.5} & \textbf{25.7} & \textbf{12.9} & \textbf{16.1} & \textbf{27.9} \\

\bottomrule
\end{tabular}%
}

\caption{Experiments with different MLLMs on the ANDH dataset.}
\label{tab:4}
\end{table}

\section{Results of different Models in the Parse Stage}
The parsing stage relies solely on textual instructions without visual input. Therefore, a text-only LLM is more appropriate, as it avoids cross-modal interference and focuses on linguistic reasoning.
As shown in Table~\ref{tab:parse_model_compare}, replacing DeepSeek-V3 with Qwen-VL results in consistent performance degradation. On the Unseen Val. split of ANDH, SR drops by 4.4 \% , with similar declines in SPL and GP.
\begin{table}[!htbp]
\centering
\small
\setlength{\tabcolsep}{1.8pt}

{\setlength{\aboverulesep}{0pt}%
 \setlength{\belowrulesep}{0pt}%
\begin{tabular}{>{\centering\arraybackslash}p{2.8cm} | 
                >{\centering\arraybackslash}m{1.5cm}
                >{\centering\arraybackslash}m{1.5cm}
                >{\centering\arraybackslash}m{1.5cm}}
 \toprule
 \rowcolor{gray!10}
 \textbf{Model} & \textbf{SPL} & \textbf{SR} & \textbf{GP} \\
 \midrule
 Qwen-VL~\cite{Alibaba23}     & \textbf{17.8} & \textbf{22.6} & \textbf{39.2} \\
 Deepseek-V3~\cite{Liu24} & 15.7 & 19.2 & 22.9 \\
 \bottomrule
 \end{tabular}%
}
\caption{Comparison of Different Models in the Parse Stage}
\label{tab:parse_model_compare}
\end{table}
\section{Detailed Prompts}
\label{sec:rationale}
Tables~\ref{tab:scot_prompt} and~\ref{tab:ccot_prompt} provide detailed prompt specifications for S-CoT and C-CoT.

\section{Failure case}
Many failure cases typically arise from interference by visually similar cues.
As shown in Figure~\ref{fig:failure_case}, the dark green target building is confused with another building of a similar color, leading to trajectory drift.
\begin{figure}[t]
    \centering
    \includegraphics[width=\columnwidth]{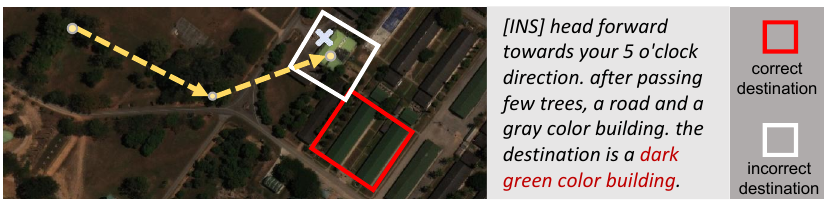}
    \caption{Failure case.}
    \label{fig:failure_case}
\end{figure}
\section{More Visualization Results}
We present additional visualization examples in Figure~\ref{fig:supp} on the ANDH and ANDH-Full datasets.
Our model can accurately interpret the given instructions, navigate to the target regions, and generate reliable navigation predictions even under challenging visual conditions.
\begin{figure*}[!h]
    \centering
    \includegraphics[width=\linewidth]{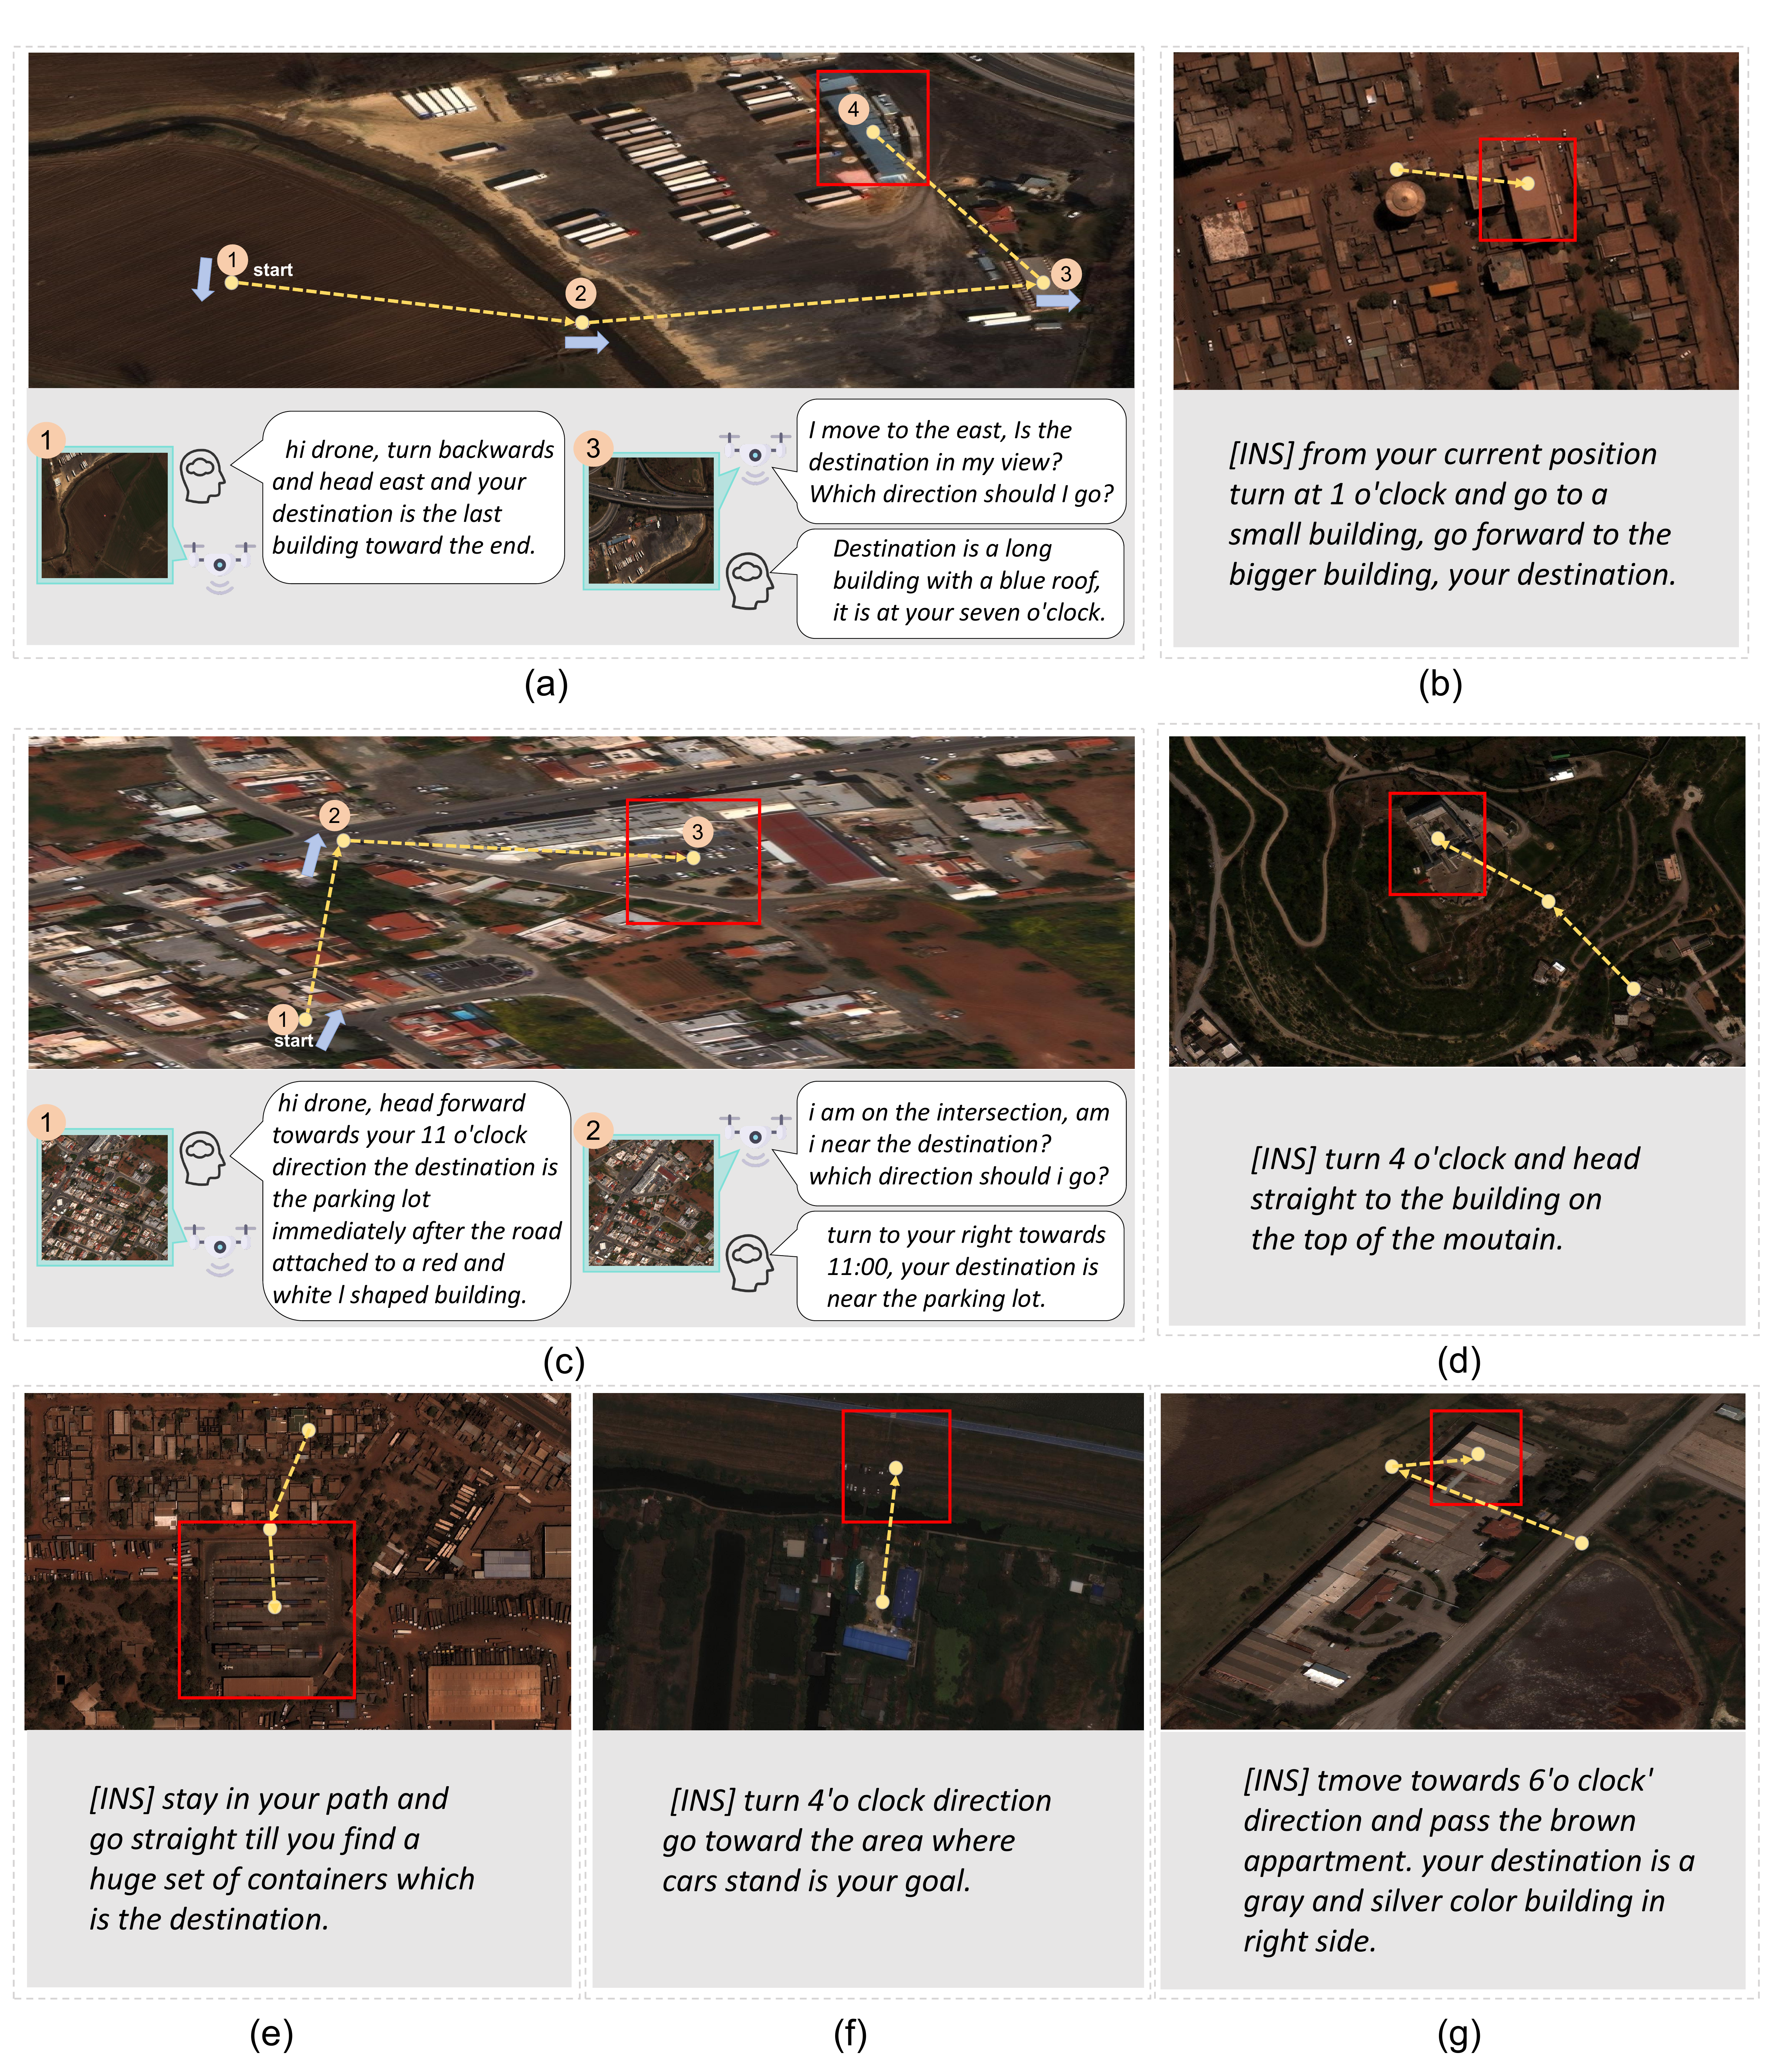}
    \caption{Additional visualization results of our method on the ANDH and ANDH-Full datasets. (a) and (c) are examples from ANDH-Full, while (b), (d), (e), (f), and (g) are examples from ANDH.}
    \label{fig:supp}
\end{figure*}
\section{Limitations}
(1) Compared with lightweight models, our MLLM-based models incur higher inference latency and token costs.
(2) Training-based approaches can leverage supervised data to achieve more concentrated navigation behavior, whereas our training-free framework lacks task-specific adaptation and is therefore more prone to error accumulation and trajectory drift, which ultimately leads to lower GP scores.

\begin{table*}[t!]\centering
\begin{minipage}{1.0\textwidth}\vspace{0mm}\centering

\begin{graylist}

{\centering \VarSty{{\bf S-CoT}}\par}
\vspace{0.6ex}

\textbf{Views:}\\
Image 1: main view (\fformat{FIXED\_CROP\_SIDE} $\times$ \fformat{FIXED\_CROP\_SIDE}), top indicates the current heading.\\
This is the only image you may output a bounding box for.\\
Image 2: same center and heading as Image~1 but with a narrower, more zoomed-in view of the same moment (local detail context).\\
Image 3: same center and heading as Image~1 but with a wider, more zoomed-out view of the same moment (broader surrounding context).\\
Image 4: north-up global map; red dot represents the current position, red arrow denotes the current heading, yellow trail shows the recent trajectory.\\[0.75ex]

\hrule
\vspace{1ex}

\textbf{1) Destination analysis:}
\begin{itemize}[leftmargin=12pt,itemsep=2pt]
    \item Analyze the destination description and extract key visual / physical attributes (shape, texture, material, color).
    \item Extract geometric structure and any directional / positional cues.
\end{itemize}

\textbf{2) Scene understanding:}
\begin{itemize}[leftmargin=12pt,itemsep=2pt]
    \item Summarize the scene and spatial layout in Image~1 (main view).
    \item Summarize local spatial / contextual structure seen in Image~2 and Image~3 (they provide tighter or wider context of the exact same place and heading).
    \item Separately summarize global position / heading / trajectory cues from Image~4.
\end{itemize}

\textbf{3) Generate 5×5 reference grid on Image 1:}
\begin{itemize}[leftmargin=12pt,itemsep=2pt]
    \item Partition Image~1 into 5 rows × 5 columns (from top to bottom, from left to right).
    \item For each cell, output a label chosen only from this closed set (lowercase; 1–2 words):  
          \fformat{road}, \fformat{building}, \fformat{container yard}, \fformat{parking}, \fformat{runway},
          \fformat{water}, \fformat{field}, \fformat{forest}, \fformat{roof}, \fformat{shadow}, \fformat{rail}, \fformat{vehicle}
          (use \fformat{unknown} if unclear).
    \item Return this grid in JSON under key \fformat{"grid\_5x5"} as a 5×5 array of strings.
\end{itemize}

\textbf{4) Target localization on Image~1 only:}
\begin{itemize}[leftmargin=12pt,itemsep=2pt]
    \item First restrict your search to the top half of Image~1 (forward / current heading direction).
    \item Propose candidate regions that satisfy the destination description, using appearance, geometry, texture, shadows, arrangement, and nearby structures.
    \item If nothing in the top half matches, extend to the full Image~1 — but the final chosen region must still come from Image~1.
    \item Choose exactly one final region. If you cannot isolate one unambiguous region, output \fformat{dest\_present = false}.
\end{itemize}

\textbf{5) Bounding box output (Image~1 only):}
\begin{itemize}[leftmargin=12pt,itemsep=2pt]
    \item Produce the minimal square bounding box fully enclosing the selected region.
    \item All bounding box coordinates must be given in Image~1’s \fformat{FIXED\_CROP\_SIDE} pixel grid.
    \item Return \fformat{dest\_present} (true/false), \fformat{bbox\_2d}, confidence in [0.0, 1.0], and a brief reason ($<$500 chars).
\end{itemize}

\textbf{Rules:}
\begin{itemize}[leftmargin=12pt,itemsep=2pt]
    \item Never output or reference a bounding box on Image~2, Image~3, or Image~4; they are context only.
    \item If not sufficiently confident in one clear match, output \fformat{dest\_present = false}.
    \item These are overhead / satellite views; rely on shape, texture, spatial layout, shadows, and stable geometry rather than raw color.
\end{itemize}

\end{graylist}

\vspace{-2mm}
\caption{Detailed S-CoT prompts.}
\label{tab:scot_prompt}
\end{minipage}
\end{table*}

\begin{table*}[t!]\centering
\begin{minipage}{1.0\textwidth}\vspace{0mm}\centering

\begin{graylist}

{\centering \VarSty{{\bf C-CoT}}\par}
\vspace{0.6ex}

\textbf{Views:}\\
Image 1: main view (\fformat{FIXED\_CROP\_SIDE} $\times$ \fformat{FIXED\_CROP\_SIDE}), top indicates the current heading.
This is the only image you may output a box for.\\
Image 2: same center and heading as Image~1 but with a narrower, more zoomed-in view of the same moment (local detail context).\\
Image 3: same center and heading as Image~1 but with a wider, more zoomed-out view of the same moment (broader surrounding context).\\
Image 4: north-up global map; red dot represents the current position, red arrow denotes the current heading, yellow trail shows the recent trajectory.\\[0.75ex]

the current heading, yellow trail shows the recent trajectory.\\[0.75ex]

\hrule
\vspace{0.6ex}

\textbf{Reasoning Chain:}\\
\textbf{Step 1} --- Generate an explicit reasoning chain. Break the destination description into ordered, checkable sub-steps. Example: ``the vehicle on the far left of the central parking line'' $\rightarrow$ ``identify the central parking line'' $\rightarrow$ ``scan along that line for the leftmost vehicle.''\\[0.25ex]

\textbf{Step 2} --- Follow those sub-steps on Image~1. For each sub-step, progressively narrow the candidate area in Image~1, starting with the top half first whenever it applies. Use Image~2 / Image~3 only to clarify local geometry and layout (e.g., which elongated strip is a runway, which dense blob is a parking lot), and use Image~4 only for high-level position / heading / trajectory context. Record at least one concrete visual evidence item for each critical sub-step.\\[0.75ex]

\textbf{Generate reference grid map on Image 1:}
\begin{itemize}[leftmargin=12pt,itemsep=2pt]
    \item Partition Image~1 into 5 rows $\times$ 5 columns (from top to bottom, from left to right).
    \item For each cell, output a label chosen only from this closed set (lowercase; 1--2 words):\\
          \fformat{road}, \fformat{building}, \fformat{container yard}, \fformat{parking}, \fformat{runway},
          \fformat{water}, \fformat{field}, \fformat{forest}, \fformat{roof}, \fformat{shadow}, \fformat{rail}, \fformat{vehicle}
          (use \fformat{unknown} if unclear).
    \item Return this grid in json under key \fformat{"grid\_5x5"} as a 5$\times$5 array of strings.
\end{itemize}

\textbf{Bounding box output:}
\begin{itemize}[leftmargin=12pt,itemsep=2pt]
    \item Draw one tight square bounding box that encloses the final chosen region on image~1 only.
    \item All bbox coordinates must be reported in Image~1's \fformat{FIXED\_CROP\_SIDE} $\times$ \fformat{FIXED\_CROP\_SIDE} pixel grid.
    \item Return \fformat{dest\_present} (true/false), \fformat{bbox\_2d}, confidence in [0.0, 1.0], and 1--3 short justification sentences.
    \begin{itemize}[leftmargin=18pt,itemsep=1pt]
        \item In Simple Direct Localization mode: name the decisive visual attributes.
        \item In Reasoning Chain mode: cite the key reasoning steps and supporting evidence.
    \end{itemize}
\end{itemize}

\hrule
\vspace{0.6ex}

\textbf{Critical rules:}
\begin{itemize}[leftmargin=12pt,itemsep=2pt]
    \item Do not output bounding boxes for Image~2, Image~3, or Image~4; they are context only.
    \item If you cannot isolate exactly one high-confidence match within Image~1, you must output \fformat{dest\_present = false}.
    \item These are overhead / satellite views; color may be low-contrast. Use structure, texture, shape, arrangement, shadows, and spatial relations, not just raw color.
\end{itemize}

\end{graylist}

\vspace{-2mm}
\caption{Detailed C-CoT prompts.}
\label{tab:ccot_prompt}
\end{minipage}
\end{table*}
